# Supplementary material for: Anomalous Thermalization in Quantum Collective Models
Source: arXiv:2003.08141 source file (2020-03-18)
Supplement: Supplementary file 1 [file supplemental.pdf]

# Supplemental material for "Anomalous thermalisation in quantum collective models"

Armando Relaño[1]

[1] *Departamento de Física Aplicada I and GISC, Universidad Complutense de Madrid, Av. Complutense s/n, 28040 Madrid, Spain**

We discuss here some details not required to follow the main text, but than can be useful for readers interested in getting a deeper insight into the calculations and some physical discussions.

## COLLECTIVE MODELS IN RECENT EXPERIMENTS

We provide here some details about the collective character of the experiments quoted in the introduction of the Letter.

A fundamental result is reported in [1]. A set of $2 \cdot 10^5$ $^{87}$Rb atoms are trapped, occupying only the ground state of the potential. Hence, the Hamiltonian consists just in the interaction term, $H = U\hat{n}\left(\hat{n}-1\right)/2$, where $\hat{n}$ is the number operator. The atomic dynamics can be aproximated by means of a semiclassical model with just one degree of freedom, $\hat{n} = \left(p^2+q^2\right)/2$. The integrability of this model is behind the main result reported in the cited paper —the fact that the system does not relax to an equilibrium state, but shows enduring collapses and revivals.

In [2], the Hamiltonian of the Lipkin-Meshkov-Glick (LMG), written here by means of angular momentum operators, $\vec{J} = (J_x, J_y, J_z)$, instead of scalar bosons as it is done in the main text, $H = \xi \hat{J}_z^{\,2} - \Omega \hat{J}_x$, is realized by means of an ensemble of $N \sim 500$ atoms. The semiclassical approximation depends on a single degree of freedom, described by the imbalance $z$ and the phase $\phi$. Non-equilibrium dynamics resulting in a classical bifurcation characterized by a kind of symmetry-breaking is observed. A two-site Bose-Hubbard model, with the same semiclassical approximation and $N \sim 1000$ atoms, is studied in [3]; again, non-equilibrium dynamics resulting in symmetry-breaking steady-states is reported. The same model, again described by just a semiclassical degree of freedom given by the imbalance $z$ and the phase $\phi$, and very similar features is covered in [4], with $N \sim 4500$ atoms. In this case, the equilibrium properties of a quantum phase transition (QPT) are analyzed.

Non-equilibrium dynamics in a generalization of the LMG model, coming from a different technique and $N \sim 4000$ atoms, is studied in [5]. The Hamiltonian is a bit more complex, but it can still be written in terms of a single collective spin, $H = -\delta \hat{S}_z - \omega \hat{S}_x + \xi \hat{S}_z^{\,2} + C(N-1)\hat{S}_z + J\vec{S}\cdot\vec{S}$. It can be approximated by a semiclassical model with just one degree of freedom. This approximation comes from the classical version of the spin, $\vec{S} = S\left(\sin\theta\cos\phi, \sin\theta\sin\phi, \cos\theta\right)$, which angular variables $(\theta,\phi)$ can be transformed into canonical coordinate and momentum, $(p,q)$.

The fluctuations of an unestable equilibrum state in a similar model is studied in [6], using an ensemble of $N \sim 40000$ atoms. In this case, the state of the system can be fully characterized by just three quantum numbers, $N_{-1}$, $N_0$, and $N_1$, stating the number of atoms in each of the three states of spin-1 particles. The Hamiltonian commutes with both $N = N_{-1} + N_0 + N_1$ and $M = N_{-1} - N_1$. Hence, the system can be understood as a set of $N$ quasi-particles created and annihilated by the corresponding operators, $b^\dagger$ and $b$, from which a single-degree of freedom classical Hamiltonian can be derived, $q = \left(b^\dagger + b\right)/\sqrt{2}$, $p = i\left(b^\dagger - b\right)/\sqrt{2}$.

Reference [7] deals with another collective model with just one semiclassical degree of freedom, obtained from $N \sim 10^5$ atoms, and including interaction $m$-body interaction terms, $H = U_2\hat{n}\left(\hat{n}-1\right)/2 + U_3\hat{n}\left(\hat{n}-1\right)\left(\hat{n}-2\right)/6 + U_4\hat{n}\left(\hat{n}-1\right)\left(\hat{n}-2\right)\left(\hat{n}-3\right)/24$, where the operator number $\hat{n}$, can be described by $\hat{n} = \left(p^2+q^2\right)/2$, when the number of atoms is large enough. Non-equilibrium dynamics after a quench is studied.

And the paradigmatic Dicke model is realized in [8], by means $N \sim 10^5$ atoms; as it is discussed in the main text, the corresponding classical model has two degrees of freedom. QPTs featuring symmetry-breaking are reported.

## CONDITION FOR THE MICROCANONICAL QUANTUM CROOK'S THEOREM

We derive here Eq. (2) of the main text, which establishes a condition for the microcanonical quantum Crook's theorem. We follow the same line of reasoning that in Ref. [9].

Let us consider a non-equilibrium process in which an external parameter of the Hamiltonian is changed from $\alpha_i$ to $\alpha_f$. If the initial condition is an eigenstate $|E_n(\alpha_i)\rangle$ of the initial Hamiltonian, $H\left(\alpha_i\right)$, with energy $E_n$, the probability of ending in an eigenstate $|E_m(\alpha_f)\rangle$ of the final Hamiltonian, $H\left(\alpha_f\right)$, with energy $E_m = E_n + w$, after a projective

measurement of the energy, is

$$p_F\left(E_n \to E_n + w\right) = \sum_m p\left[E_m(\alpha_f)|\, E_n(\alpha_i)\right] \delta\left[E_m(\alpha_f) - E_n(\alpha_i) - w\right]. \tag{1}$$

The subindex $F$ denotes that this is the forward process (in contrast with the backwards, $B$, $\alpha_f \to \alpha_i$), and $p\left[E_m(\alpha_f)|\, E_n(\alpha_i)\right]$ is the transition probability, $p\left[E_m(\alpha_f)|\, E_n(\alpha_i)\right] = \left|\langle E_m(\alpha_f)|\, U(t)\, |E_n(\alpha_i)\rangle\right|^2$, being $U(t)$ the time-evolution operator, which depends on the *trajectory* followed by the process. For a single quench —a sudden change from $\alpha_i$ to $\alpha_f$— the time-evolution operator just depends on the final Hamiltonian, $U(t) = \exp\left[-iH\left(\alpha_f\right)t\right]$. Hence, the calculation of the transition probabilities is straightforward if we express the eigenstates of the initial Hamiltonian in an eigenbasis of the final one, $|E_n\left(\alpha_i\right)\rangle = \sum_k C_k^n\, |E_k\left(\alpha_f\right)\rangle$, where $C_k^n = \langle E_n\left(\alpha_i\right)|\, E_k\left(\alpha_f\right)\rangle$,

$$\langle E_m(\alpha_f)|\, U(t)\, |E_n(\alpha_i)\rangle = \langle E_m\left(\alpha_f\right)| \sum_k C_k^n \exp\left[-iE_k\left(\alpha_f\right)t\right] |E_k\left(\alpha_f\right)\rangle = C_m^n \exp\left[-iE_m\left(\alpha_f\right)\right]. \tag{2}$$

Thus,

$$p\left[E_m(\alpha_f)|\, E_n(\alpha_i)\right] = \left|C_m^n\right|^2. \tag{3}$$

The results for the LMG model in the main text are obtained using single quenches as non-equilibrium protocols. On the contrary, trajectories are a bit more complicated in the numerical experiments with the Dicke model.

Now, let us assume that the transitions probabilities, $p\left[E_m(\alpha_f)|\, E_n(\alpha_i)\right]$, are smooth functions of the final energy. This is expected to happen in chaotic systems, in which there are no conserved charges precluding certain transitions [9]; the probabilities $\left|C_m^n\right|^2$ are supposed to randomly fluctuate around an energy-dependent average value, if the system is fully chaotic or ergodic [10]. Then, if we consider that the measured work, $w$, is not the exact (and microscopic) energy difference between eigenstates, but a macroscopic magnitude $w \pm \Delta w$, where $\Delta w$ includes a large number of energy levels, we can change the sum in Eq. (1) by an integral

$$p_F\left(E_n \to E_n + w\right) = \int dx\, g(x, \alpha_f) p\left[x|\, E_n(\alpha_i)\right] \delta\left[x - E_n(\alpha_i) - w\right] = g(E_n(\alpha_i) + w, \alpha_f) p\left[E_n(\alpha_i) + w|\, E_n(\alpha_i)\right]. \tag{4}$$

where $g(x, \alpha_f)$ is the density of states of the final Hamiltonian, $H(\alpha_f)$.

Applying the same reasoning to the backward part of the process, we obtain

$$p_B\left(E_n + w \to E_n\right) = g(E_n(\alpha_i), \alpha_i) p\left[E_n(\alpha_i)|\, E_n(\alpha_i) + w\right]. \tag{5}$$

Finally, considering microrreversibility, $p\left[E_n(\alpha_i) + w|\, E_n(\alpha_i)\right] = p\left[E_n(\alpha_i)|\, E_n(\alpha_i) + w\right]$, we recover Eq. (1) of the main text

$$\frac{P_f(E, \alpha_i, w)}{P_b(E + w, \alpha_f, -w)} = \frac{g(E + w, \alpha_f)}{g(E, \alpha_i)}. \tag{6}$$

As the density of states typically increases with energy, this equality reflects that any non-equilibrium process entails an irreversible loss of work, which is transformed into thermal energy.

Let us now imagine that the initial state of the process is not an eigenstate, but a mixture described by a density matrix $\rho_i = \sum_n p_n\, |E_n(\alpha_i)\rangle\, \langle E_n(\alpha_i)|$. Then, the probability that a certain amount of work, $w$, is required to complete the forward part of the process is

$$p_F\left(E \to E + w\right) = \sum_n p_n p_F\left(E_n(\alpha_i) \to E_n(\alpha_i) + w\right) = \sum_n p_n g(E_n(\alpha_i) + w, \alpha_f) p\left[E_n(\alpha_i) + w|\, E_n(\alpha_i)\right], \tag{7}$$

where $E$ is the expected value for the energy, $E = \sum_n p_n E_n$.

Finally, let us consider that the initial state is narrow in the eigenbasis $\{|E_n(\alpha_i)\rangle\}$. Then, we can expand both the density of states and the transition probabilities around the expected energy $E$. Denoting $x_n = E - E_n$, we get

$$g(E_n(\alpha_i) + w, \alpha_f) = g(E + w, \alpha_f) + \frac{\partial g}{\partial E} x_n + \frac{1}{2} \frac{\partial^2 g}{\partial E^2} x_n^2 + O(x_n^3), \tag{8}$$

$$p\left[E_n(\alpha_i) + w|\, E_n(\alpha_i)\right] = p\left[E + w|\, E\right] + \frac{\partial p}{\partial E} x_n + \frac{1}{2} \frac{\partial^2 p}{\partial E^2} x_n^2 + O(x_n^3). \tag{9}$$

As a consequence, we obtain

$$p_F\left(E\to E+w\right)=g(E+w,\alpha_f)p\left[E+w|\;E\right]+g(E+w,\alpha_f)\frac{\partial p}{\partial E}\sum_n p_nx_n+p\left[E+w|\;E\right]\frac{\partial g}{\partial E}\sum_n p_nx_n+ \\ +\frac{1}{2}g(E+w,\alpha_f)\frac{\partial^2 p}{\partial E^2}\sum_n p_nx_n^2+\frac{1}{2}p\left[E+w|\;E\right]\frac{\partial^2 g}{\partial E^2}\sum_n p_nx_n^2+\frac{\partial g}{\partial E}\frac{\partial p}{\partial E}\sum_n p_nx_n^2+O(x_n^3). \tag{10}$$

And, taking into account that $\sum_n p_nx_n=0$, we finally get

$$p_F\left(E\to E+w\right)=g(E+w,\alpha_f)p\left[E+w|\;E\right]+\frac{1}{2}\sum_n p_nx_n^2\left[g(E+w,\alpha_f)p''(E)+p\left[E+w|\;E\right]g''(E)+p'(E)g'(E)\right], \tag{11}$$

up to $O(x_n^3)$.

As the result for the backward part of the process is the same, Eq. (6) holds for an initial condition $\rho_i=\sum_n p_n\left|E_n(\alpha_i)\right\rangle\left\langle E_n(\alpha_i)\right|$ if the second-order correction in Eq. (11) is small enought, that is, if

$$\left|g''(E)/g(E)+P''(E)/P(E)+P'(E)g'(E)/\left[P(E)g(E)\right]\right|(\Delta E)^2\ll 1, \tag{12}$$

where $(\Delta E)^2$ is the energy width of the initial state, $(\Delta E)^2=\sum_n p_nx_n^2=\sum_n p_n\left(E-E_n\right)^2$. This is the main theoretical result shown in Eq. (2) of the main text.

As it is pointed there, Eq. (12), imposses conditions on the density of states and the transition probabilities, both including first and second derivatives of these magnitudes. That is, to apply Eq. (6) to any non-equilibrium process $\alpha_i\to\alpha_f$ is required that the initial state is very narrow in energy. If not, the assymetry between the forward and the backward parts of the process depends on the actual shape of the initial state, given by the probabilities $p_n$. This implies that different initial states with the same expected energy $E$ can give rise to different work statistics for the same process $\alpha(t)$, and that different processes $\alpha(t)$ covering $\alpha_i\to\alpha_f$ can also give rise to different work statistics. A remarkable consequence of Eq. (12) is that, due to its dependence on the transition probabilities, $P(E)$, this condition might be more or less demanding depending on what trajectory follows the non-equilibrium protocol. Hence, to be sure that the quantum microcanonical Crook's theorem holds in any case, the initial state must be very narrow in energy.

It is worth noting that, even though Eq. 12) is not obtained from a pure initial state, $\left|\psi(0)\right\rangle=\sum_n C_n\left|E_n\left(\alpha_i\right)\right\rangle$, but for an initial density matrix, $\rho(0)=\sum_n p_n\left|E_n\left(\alpha_i\right)\right\rangle\left\langle E_n\left(\alpha_i\right)\right|$, the same final result holds for an initial pure state with $p_n=\left|C_n\right|^2$ if a two-projective measurement scheme is used, as it is done in all the numerical experiments discussed in the main text. The consequences of performing non-equilibrium processes from initial pure states, without any previous energy measurement, are not relevant for this work [11].

## SEMICLASSICAL CALCULATIONS

### The LMG model

As is pointed in the main text, the LMG model can be described by meanso of the following classical Hamiltonian, in the thermodynamic limit, $N\to\infty$,

$$H(q,p)=\alpha p^2+(5\alpha-4)\,p\,(1-p)-4\,(1-\alpha)\,p\,(1-p)\sin^2 q, \tag{13}$$

where $0\le\alpha\le 1$. The canonical coordinates $(p,q)$ are restricted to $0\le p\le 1$, and $-\pi\le q\le\pi$. The semiclassical energy $H(q,p)=E$ coincides with the quantum energy per particle, $E/N$, in the thermodynamical limit; we refer to this normalised energy throughout all this text. As Hamiltonian (13) has just one degree of freedom, it is integrable; however, its trejectories are also ergodic under certain circumstances. More details about these facts can be found in references [12–15].

Microcanonical averages can be obtained from Eq. (13). The first step of the procedure consists in calculating the density of states,

$$g(E)=\int dq dp\,\delta\left[H(q,p)-E\right]. \tag{14}$$

The integral over the variable $p$ can be done analytically. Considering that $\delta(f[x]) = \sum_{x_0} \delta\left(x - x_0\right) / \left|f'(x_0)\right|$, where $f(x_0) = 0$, we obtain

$$g(E) = \int_{q_-}^{q_+} dq \left[ \frac{1}{\left| H_p(p_+(E), q) \right|} + \frac{1}{\left| H_p(p_-(E), q) \right|} \right], \tag{15}$$

where $H_p(p, q) = \partial H / \partial p$, and

$$p_\pm(E) = \frac{1}{8(\alpha - 1)} \left[ -4 + \alpha \left( 4 + \frac{1}{\cos^2 q} \right) \pm \frac{1}{\cos^2 q} \sqrt{\left( 4 - 5\alpha + 4(\alpha - 1)\sin^2 q \right)^2 + 16(1 - \alpha) E \cos^2 q} \right], \tag{16}$$

iff

$$\left( 4 - 5\alpha + 4(\alpha - 1)\sin^2 q \right)^2 + 16(1 - \alpha) E \cos^2 q \geq 0. \tag{17}$$

If this condition is not fulfilled, $g(E) = 0$.

The second integral does not admit a general solution in terms of simple functions. To proceed forward we restrict ourselves to $0 \leq \alpha < 4/5$. At $\alpha_c = 4/5$ there exists a quantum phase transition (QPT), separating the *normal* phase, $\alpha > 4/5$, and the *deformed* (or symmetry-broken) phase, $\alpha < 4/5$, [12]. In the last one, there exists also an excited-state quantum phase transition (ESQPT), at the critical energy $E_c = 0$ [13]. Below this energy, all the quantum energy levels are degenerate in pairs, and eigenstates in which the parity symmetry is broken also exist. The reader interested in this feature and its consequences can refer to [13–15]. The corresponding classical contour curves of constant energy, $H(q, p) = E$, are disjoint. As a consequence, the integral (15) has to be splitted in two parts. However, both of these parts give the same results for the density of states, $g(E)$, and for microcanonical averages of observables that do not break the parity symmetry; hence, we can restrict ourselves to one of the parts, and multiply the final result by a factor two. On the other hand, if $E > 0$, there exists just one connected region for the curve $H(q, p) = E$, and therefore the corresponding integral can be completed in just one step.

From all these considerations, we can derive the lower and upper limits of the integral in Eq. (15). If $E > 0$, the contour curve covers all the possible values of the position $q$, and thus $q_- = -\pi$ and $q_+ = \pi$. On the contrary, if $E < 0$ the values of $q$ are restricted by the condition (17). Considering that $q$ is periodic, we obtain

$$q_- = f \left[ \sqrt{\frac{-\alpha + 2E - 2\sqrt{E(E - \alpha)}}{\alpha - 1}}, \sqrt{\frac{-4 + 5\alpha - 2E + 2\sqrt{E(E - \alpha)}}{\alpha - 1}} \right], \tag{18}$$

$$q_+ = f \left[ \sqrt{(1 - \alpha)(\alpha - 2E) + 2\sqrt{E(E - \alpha)}(1 - \alpha)}, \sqrt{(\alpha - 1)(-4 + 5\alpha - 2E) - 2\sqrt{E(E - \alpha)}(1 - \alpha)} \right], \tag{19}$$

where $f(x, y)$ denotes that $\sin q = x$ and $\cos q = y$. That is, the function $f(x, y)$ is like $\operatorname{atan}(y/x)$, but explicitely taking into account the cuadrant of the angle.

All the calculations performed in the main part of the paper are completed following this procedure, and doing numerically the last integration. As an example, we plot in Fig. 1 the results for $\alpha = 0.5$. We can see a singularity located at the critical energy $E_c = 0$, as is expected for an ESQPT. The presence of this singularity is the reason why we avoid this region in all the numerical experiments discussed in the main text.

The calculation of microcanonical averages,

$$\langle \mathcal{O}(E) \rangle = \frac{1}{g(E)} \int dq dp\, \mathcal{O}(p, q) \delta\left[ E - H(q, p) \right], \tag{20}$$

is done following the same procedure, taking into account that $n_t/N = p$, $n_t^2/N^2 = p^2$, $n_t n_s = p(1 - p)/N^2$, and $Q \cdot Q / N^2 = 4p(1 - p)\cos^2 q$. It is worth noting that none of these observables breaks the parity symmetry, and thus the average can be safely done using just one of the two parts of the disjoint contour curves of constant energy. Results are summarized in Fig. 2, again for $\alpha = 0.5$. We can see abrupt dips at the critical energy $E_c$. As a consequence, thermalisation is expected to be problematic if the energy is close to $E_c$; as $\mathcal{O}''(E)$ is not well-defined around the critical energy, the condition for thermalisation, $(\Delta E)^2 \left| \mathcal{O}''(E) / \mathcal{O}(E) \right| \ll 1$, is not fulfilled at all. Nevertheless, this does not constituite a problem for our calculations, since we have avoided this region, both to study thermalisation, and to test the microcanonical quantum fluctuiation theorem.

Before ending this section, a brief comment about the classical version of the LMG model, Eq. (13), is worthy. Having just one degree of freedom entails that all the trajectories are periodic. As a consequence, and although the results

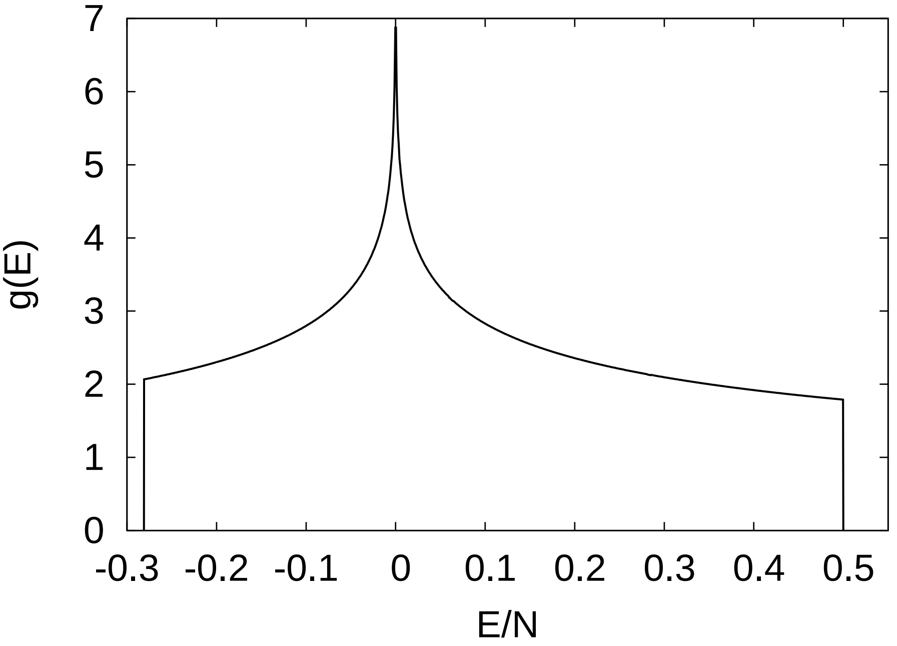


FIG. 1. Density of states of the LMG model with $\alpha = 0.5$

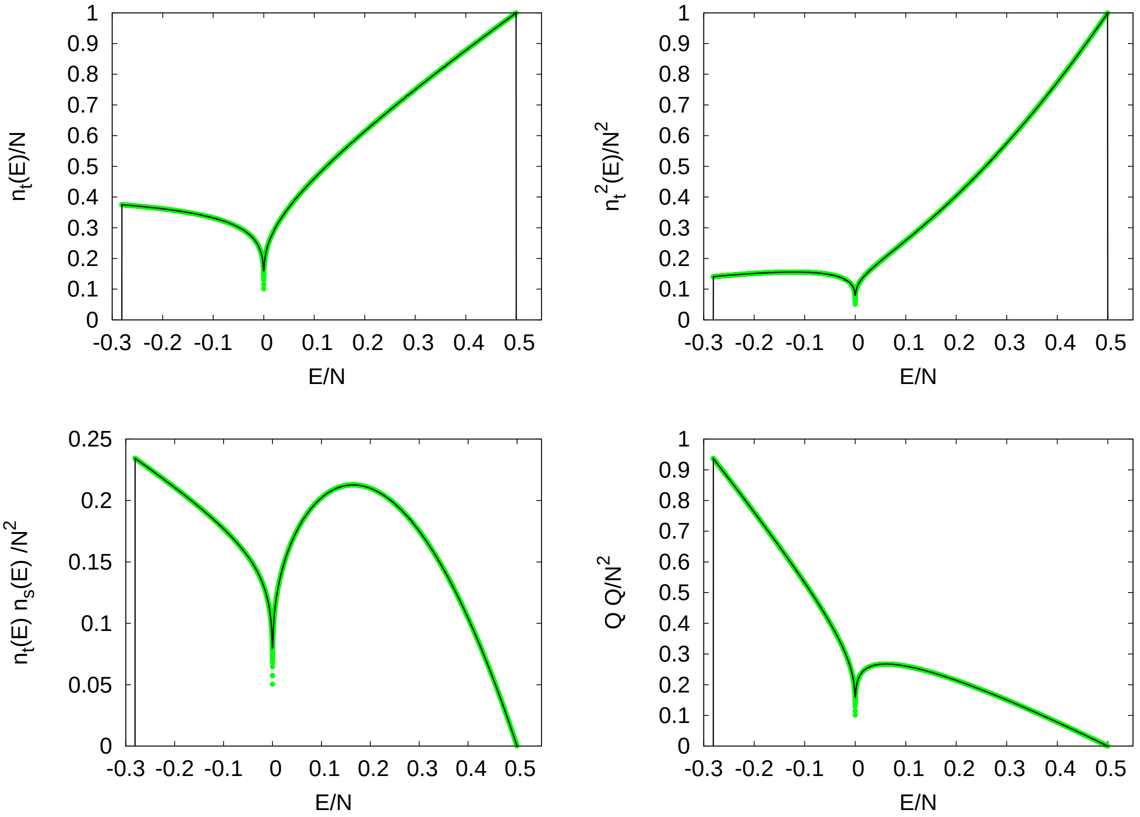


FIG. 2. Black lines, microcanonical averages of the four observables studied in the main text for the LMG model, $n_t/N$ (upper left), $n_t^2/N^2$ (upper right), $n_t n_s/N^2$ (lower left) and $Q \cdot Q/N^2$ (lower right). Green points, expected values of the same observables in all the eigenstates, $\langle E_n | \mathcal{O} | E_n \rangle$, as a function of the energy. In all the cases $\alpha = 0.5$.

shown in Fig. 2 correctly account for long-time averages of classical observables, $\langle \mathcal{O} \rangle = \lim_{T\to\infty}(1/T)\int_0^T dt\, \mathcal{O}(t)$, we cannot say that the classical version of the LMG equilibrates; the exact time-dependent values for the observables, $\mathcal{O}(t)$, periodically and smoothly oscillate around the average $\langle \mathcal{O} \rangle$. However, in quantum mechanics the situation is rather different. The exact time-dependent expected value of any observable $\mathcal{O}(t)$ is

$$\langle \mathcal{O}(t) \rangle = \sum_{n,m} C_m^* C_n \mathrm{e}^{-i(E_n - E_m)t} \langle E_n | \mathcal{O} | E_m \rangle \,, \tag{21}$$

where $|E_n\rangle$ is the eigenstate with energy $E_n$, $C_n = \langle \psi(0) | E_n \rangle$, and $|\psi(0)\rangle$ is the initial state. Hence, periodicity of the quantum evolution depends on the gaps between levels, $E_n - E_m$; the period $T$ is the minimum time for which $(E_n - E_m)\,T = 2\pi k$, $\forall n, m$ and $k \in \mathbb{Z}$. As a consequencue, due to the fact that many different energy levels are effectively populated in our numerical experiments (data are given in the main part of the manuscript), this periodicity would happen for extremely large times, and hence we can consider that the quantum dynamics is not periodic at all. Results given in the main text, showing that the size of the fluctuations around $\langle \mathcal{O} \rangle$ descrease with the number of atoms, $N$, corroborate this conclusion.

**The Dicke model**

There are several strategies to build a semiclassical description of the Dicke model. We follow here the one discussed in [16]. The corresponding classical Hamiltonian, valid in the thermodynamic limit $j \to \infty$, is

$$H(q,p;jz,\phi) = \omega_o j_z + \frac{\omega}{2}\left(q^2 + p^2\right) + 2\alpha\sqrt{j}\sqrt{1 - \frac{jz^2}{j^2}}\cos\phi, \tag{22}$$

where $(q,p)$ are the coordinate and the momentum of the monochromatic radiation field, and $(\phi, j_z)$, the corresponding to the set of $N$ atoms ($N = 2j$).

A classical system with two degrees of freedom requires two independent integrals of motion in involution to be integrable. It has been recently shown that the Dicke model has an approximate second integral of motion in the low-energy region [17]. But, contrary to what happens in the LMG model, it is generically chaotic. A recent analysis of quantum chaos in the Dicke model is done in [18].

The density of the states can be calculated as follows

$$g(E) = \frac{1}{(2\pi)^2}\int dq dp d\phi dj_z \, \delta\left[H(q,p;\phi j_z) - E\right], \tag{23}$$

where the factor $1/(2\pi)^2$ comes from the measure $d\phi dj_z$. The variable $q$ can be integrated following the same method that for the LMG model. The result is

$$g(E) = \frac{1}{2\pi^2}\int dp d\phi dj_z \, \frac{1}{\sqrt{c - \omega^2 p^2}}, \tag{24}$$

where $c = 2\alpha^2 j\left(1 - j_z^2/j^2\right)\cos^2\phi + 2\omega\left(E - \omega_o j_z\right)$.

The integral in $p$ can be performed considering that $c \geq \omega^2 p^2$. The result is

$$g(E) = \frac{1}{2\pi\omega}\int d\phi dj_z, \tag{25}$$

if the following condition is fulfilled

$$\frac{2\alpha^2}{\omega\omega_o}\left(1 - \frac{j_z^2}{j^2}\right)\cos^2\phi \geq \frac{j_z}{j} - \frac{E}{\omega_o j}. \tag{26}$$

So, despite the simple shape of Eq. (25), the actual expression for the density of states is highly involved. Eq. (26) establishes the range of the atomic variables, $(\phi, j_z)$, as a function of the energy $E$. To proceed further we restrict ourselves to the superradiant phase, $\alpha \geq \sqrt{\omega\omega_o}/2$, where an excited-state quantum phase transition takes place at $E_c = -\omega_o j$. As it happens in the LMG model, below this energy all the levels are degenerate in pairs, and the surfaces of constant energy are disjoint in the phase space; above $E_c$, there is just one connected region. Eq. (26) summarizes

these facts. Its consequences, in terms of precise integration limits, are very complex. Thus, we refer the reader interested in more details to reference [16]. Here, we give the final result for the superradiant phase, $\alpha \geq \sqrt{\omega\omega_o}/2$, in which all the numerical experiments discussed in the main text are performed,

$$g(E) = \begin{cases} \dfrac{2j}{\omega\pi}\displaystyle\int_{y_-}^{y_+} \arccos\sqrt{\dfrac{\omega\omega_o\left(y-\frac{E}{\omega_o j}\right)}{\alpha^2\left(1-y^2\right)}}, \; E_0 \geq E < -\omega_o j, \\ \dfrac{E+\omega_o j}{\omega\omega_o} + \dfrac{2j}{\omega\pi}\displaystyle\int_{\frac{E}{\omega_o j}}^{y_+} \arccos\sqrt{\dfrac{\omega\omega_o\left(y-\frac{E}{\omega_o j}\right)}{\alpha^2\left(1-y^2\right)}}, \; -\omega_o j \geq E < \omega_o j, \\ \dfrac{2j}{\omega}, \; E > \omega_o j, \end{cases} \tag{27}$$

where $E_0$ is the ground-state energy, and

$$y_{\pm} = \left[ -\frac{\omega\omega_o}{4\alpha^2} \pm \sqrt{\frac{\omega\omega_o}{2\alpha}\sqrt{2\left(\frac{E-E_0}{\omega_o j}\right)}} \right]. \tag{28}$$

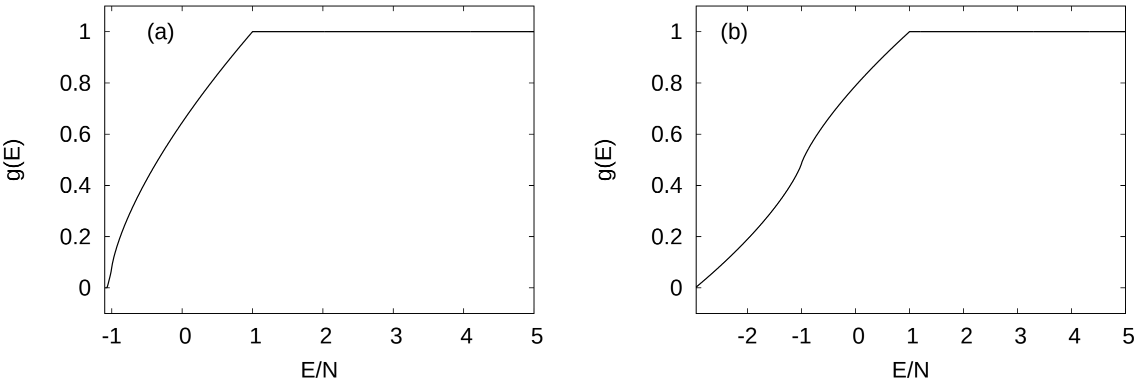


FIG. 3. Panel (a), density of states of the Dicke model with $\omega = \omega_o = 1$ and $\alpha = 0.6$. Panel (b), density of states of the Dicke model with $\omega = \omega_o = 1$ and $\alpha = 1.2$.

The density of states of the Dicke model is shown in Fig. 3, for $\omega = \omega_o = 1$ and $\alpha = 0.6$ (panel (a)), and $\alpha = 1.2$ (panel(b)). In the first case, the critical energy of the ESQPT is very close to the ground state; no traces of it are visible in the Figure. In the second case, we can see a subtle curvature change at $E/j = -1$, a much weaker signature of an ESQPT than in the LMG model. This is a consequence of the second degree of freedom. We refere the reader to [19] for more details. The interpretation of the non-analytical point at $E/j = 1$ is controversial [20, 21]. Above this point, the dynamics of the atomic part of the system, described by $(j_z/j\phi)$, covers its whole phase space.

Analytical microcanonical averages can be obtained following the same strategy, although the shape of the integrals becomes more involved, specially for observables related to the radiation field. However, we do not work with analytical microcanonical averages in the main text. The reason is that the number of atoms, $N = 50$, is not large enough to avoid finite-size effects. Thermalisation for observables is tested comparing long-time with quantum microcanonical averages. In Figs. 4 and 5, we show the expected values of the observables discussed in the main text (see captions of the figures for details) together with the quantum microcanonical averages over 51 eigenstates, for $\omega = \omega_o = 1$ and both $\alpha = 0.6$ and $\alpha = 1.2$. In the first case, all the expected values in any eigenstate fluctuate around the microcanonical averages; fluctuations are large due to the small number of atoms, but the microcanonical average provides the right mean value. The second case is different. Above $E/j \sim -1$, the behaviour is the same than in the case with $\alpha = 0.6$. Below, we see that the plot is arranged in bands, specially for the observables $a^\dagger a$, and $\left(a^\dagger + a\right)^2$. This is a consequence of the integrable character of the Dicke model at low energies [17]. Due to the second integral of motion, the classsical trajectories do not cover the whole energy surface; they are restricted by the value of this second integral. As a consequence, the condition for thermalisation is not fulfilled in this region —both $a^\dagger a(E)$ and $\left(a^\dagger + a\right)(E)$ are not smooth functions of the energy—, and hence the system is not expected to thermalise. All the

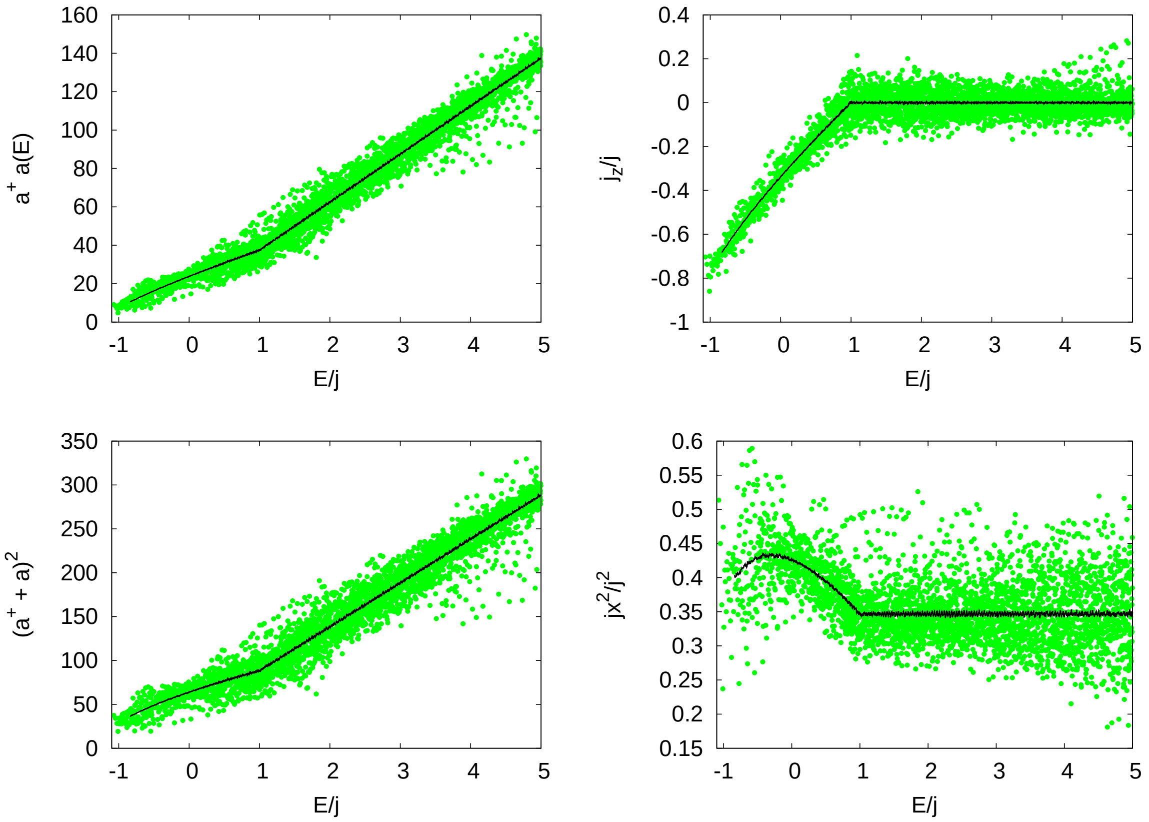


FIG. 4. Black lines, quantum microcanonical averages, using a window with $N = 51$ around the average energy, of the four observables studied in the main text, $a^\dagger a$ (upper left), $j_z/j$ (upper right), $\left(a^\dagger + a\right)^2$ (lower left) and $j_x^2/j^2$ (lower right), for the Dicke model. Green points, expected values of the same observables in all the eigenstates, $\langle E_n | \mathcal{O} | E_n \rangle$, as a function of the energy. In all the cases $\omega = \omega_o = 1$ and $\alpha = 0.6$.

numerical experiments discussed in the main text are performed above this integrable region. In particular, all the non-equilibrium processes, $\alpha = 1.2 \rightarrow \alpha = 0.6$ start from $E/j = -0.12$, a value around which the microcanonical average works pretty well for all the observables.

## PREPARATION OF THE EQUILIBRIUM STATES

In this section we discuss the procedures used to prepare the initial states for both the LMG and the Dicke models.

### LMG model

In the main text, we have shown that two different procedures resulting in equilibrium states with the same values for the energy, $E$, and the external parameter, $\alpha$, give rise to different work statistics. As this is the main numerical result of the Letter, we provide here a detailed discussions of both procedures. The study of thermalisation is done in the following section.

#### *Procedure (i)*

This procedure consists in a simple quench giving the system the desired amount of energy:

*(i)* We cool the system to $T \rightarrow 0$ for an initial value of the external parameter, $\alpha_{\text{ini}}$. In other words, we lead the system onto its ground state.

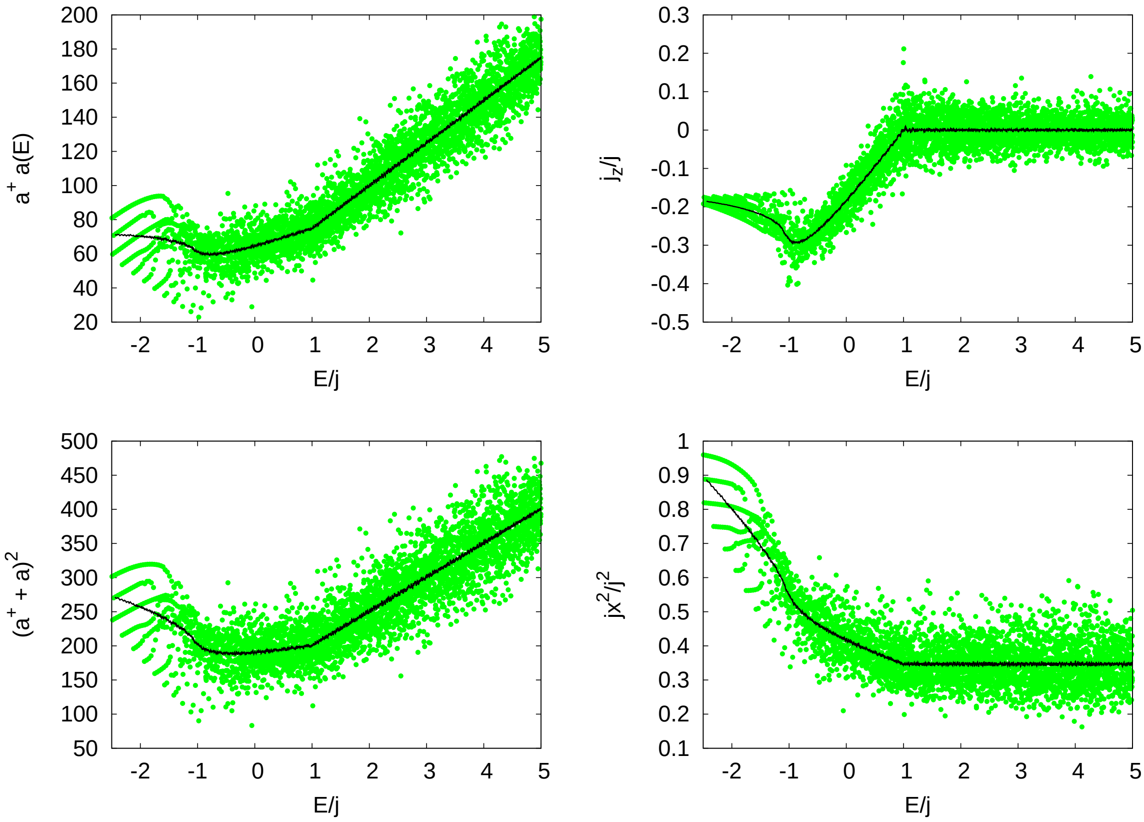


FIG. 5. Black lines, quantum microcanonical averages, using a window with $N = 51$ around the average energy, of the four observables studied in the main text, $a^\dagger a$ (upper left), $j_z/j$ (upper right), $\left(a^\dagger + a\right)^2$ (lower left) and $j_x^2/j^2$ (lower right), for the Dicke model. Green points, expected values of the same observables in all the eigenstates, $\langle E_n | \mathcal{O} | E_n \rangle$, as a function of the energy. In all the cases $\omega = \omega_o = 1$ and $\alpha = 1.2$.

*(ii)* We quench the system onto the final vaule of the external parameter, $\alpha$.

Numerically, this is a very simple procedure that can be done just by obtaining the ground state of the initial Hamiltonian, $H(\alpha_{\text{ini}})$, and letting it evolve under the final Hamiltonian, $H(\alpha)$. The values of $\alpha_{\text{ini}}$ required to reach the desired values of the energy are easily obtained from the semiclassical calculation discussed in the previous section. If $\alpha \leq 4/5$, the energy has two minima, each one coming from the corresponding part of the disjoint constant energy curves,

$$(p_{\min}, q_{\min}) = (\frac{5\alpha - 4}{8\,(\alpha - 1)}, 0), \text{ and } \quad (p_{\min}, q_{\min}) = (\frac{5\alpha - 4}{8\,(\alpha - 1)}, \pi). \tag{29}$$

In both of them, the energy is

$$E_{\min}(\alpha) = \frac{(5\alpha - 4)^2}{16\,(\alpha - 1)}. \tag{30}$$

If $\alpha > 4/5$, the only minimum is located at $(p_{\min}, q_{\min}) = (0, 0)$, and its energy is $E_{\min} = 0$.

From these results, the energy of the state resulting from the quench $\alpha_{\text{ini}} \to \alpha$ is easily obtained. If $0 \leq \alpha \leq 4/5$ and $0 \leq \alpha_{\text{ini}} \leq 4/5$,

$$E(\alpha_{\text{ini}} \to \alpha) = H\left[p_{\min}(\alpha_{\text{ini}}), q_{\min}(\alpha_{\text{ini}}), \alpha\right] = \frac{(5\alpha_{\text{ini}} - 4)\,(4 - 6\alpha + \alpha_{\text{ini}}\,[5\alpha - 3])}{16\,(\alpha_{\text{ini}} - 1)^2}. \tag{31}$$

Therefore, our numerical procedure consists in:

*(i)* Selecting the desired energy, $E$.

*(ii)* Calculating the initial value of the external parameter, $\alpha_{\text{ini}}$, from Eq. (31).

*(iii)* Obtaining the ground state of the corresponding Hamiltonian.

*(iv)* Performing the quench.

As the parity, $\Pi = (-1)^{n_t}$, is a conserved quantity, all our calculations are restricted to the sector of positive parity. Notwithstanding, our results are totally general because none of the observables we have studied break this symmetry.

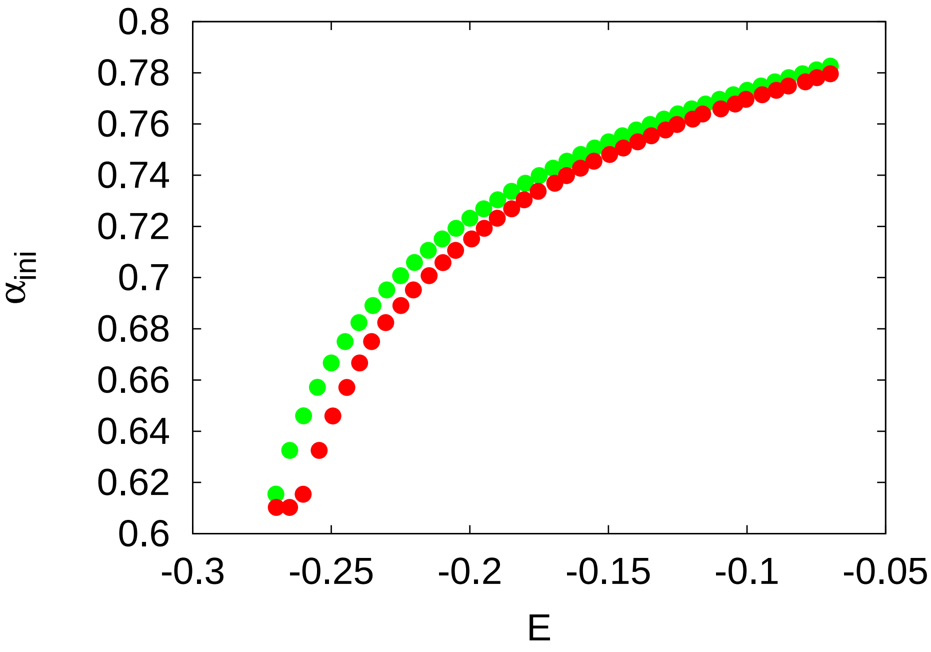


FIG. 6. Values of $\alpha_{\text{ini}}$ for both the procedure (i) (green circles) and procedure (ii) (red circles), both corresponding to numerical experiments with the LMG model, as a function of the final energy $E$, for all the cases with $\alpha = 0.5$. In all the cases, $N = 1,6{\cdot}10^4$.

In Fig. 6 we summarize the information about the quenches done for the cases with $\alpha = 0.5$ (green circles). We plot the value of $\alpha_{\text{ini}}$ required to reach the desired energy, $E$. The average distance between the desired and the obtained energies is $\Delta E \sim 2 \cdot 10^{-5}$, so the error is negligible in all the cases.

*Procedure (ii)*

The second procedure consists in repeteadly quenching the system between two different values of the external parameter, $\alpha_{\text{int}}$ and $\alpha$, to give the system the same amount of energy that with procedure (i). This procedure is a bit more complicated, and involves the following steps:

*(i)* We cool the system to $T \to 0$ for an initial value of the external parameter, $\alpha_{\text{ini}}$.

*(ii)* We quench the system onto an intermediate vaule of the external parameter, $\alpha_{\text{int}}$.

*(iii)* We let the system relax in this intermediate stage during a time $\tau = 10^8$ in the natural units of the problem (this time is large enough to assure equilibration).

*(iv)* We quench the system onto the final value of the external parameter, $\alpha$.

*(v)* We let the system relax during the same time, $\tau = 10^8$.

At this stage, we test the energy of the system. If it is above the desired energy, we stop the process and we consider that the obtained state is the right one. On the contrary, we quench back the system onto the intermediate value of the external parameter, $\alpha_{\text{int}}$, and we repeat the stages (ii)-(v).

All the parameters of this procedure have been chosen to obtain a good value for the final energy. In particular, $\alpha_{\text{int}}$ is always very close to $\alpha$; in this way, the steps (ii)-(v) give the system just a small amount of energy, and therefore the final value of the energy is close to the desired one. In particular, $\alpha_{\text{int}} = 0.53$ when $\alpha = 0.5$, and $\alpha_{\text{int}} = 0.25$ when $\alpha = 0.2$. In both cases, $\alpha_{\text{ini}}$ is chosen to lead the system to an equilibrated state with energy $E - 0.01$, being $E$ the desired energy, at stage (ii).

Values of $\alpha_{\text{ini}}$ are shown with red circles in Fig. 6, for the case with $\alpha = 0.5$, as a function of the final energy $E$ (red circles). The average distance between the desired and the obtained energies is $\Delta E \sim 3 \cdot 10^{-4}$. This distance is larger than the one obtained with procedure (i), but one order of magnitude smaller than the distance between two consecutive values of final energies, $\delta E = 5 \cdot 10^{-3}$.

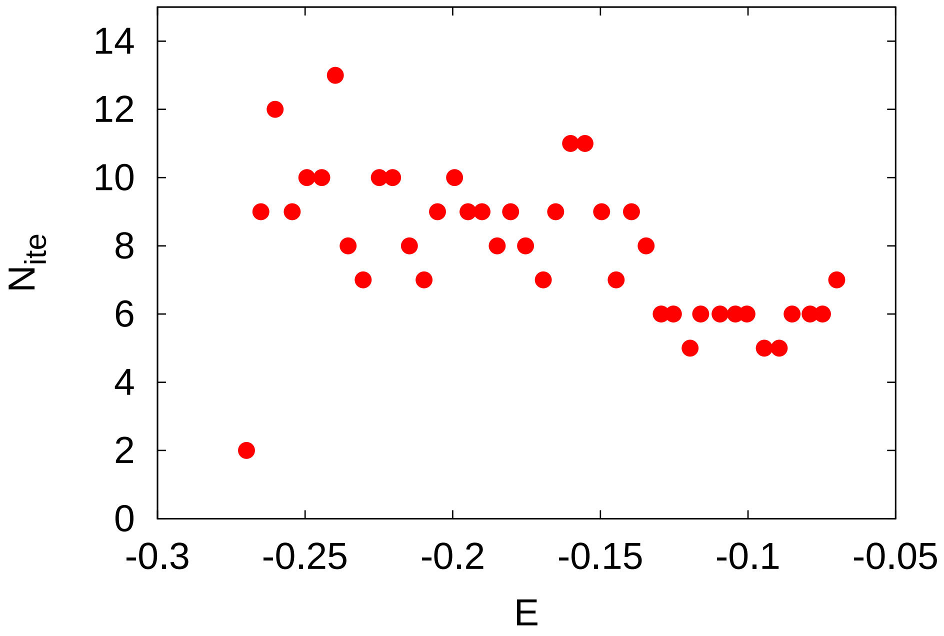


FIG. 7. Number of iterations (stages (ii)-(v)) required to reach the final energy, in numerical experiments following procedure (ii) with the LMG model. In all the cases, $\alpha = 0.5$ and $N = 1,6 \cdot 10^4$.

The number of iterations required to reach the final energy (that is, the number of times stages (ii)-(v) are repeated) are summarized in Fig. 7, for the case with $\alpha = 0.5$ and $N = 1,6 \cdot 10^4$. Fluctuations are large because the amount of energy given for each of the intermediate quenches, $\alpha \to \alpha_{\text{int}} \to \alpha$, is quite random. In any case, we can conclude that a small number of such quenches is enough to obtain an energy distribution totally different from the one coming from procedure (i). It is worth noting that just one iteration is enough to produce a wide and erratic final energy distribution, like the ones displayed in panel (a) of Fig. 4 of the main text. The cause of this fact is the following. If we perform just a single quench from the ground state of $H(\alpha_{\text{ini}})$, the time during which the system evolves under the initial Hamiltonian is irrelevant; this time evolution only introduces a global phase in the wavefunction, $|\psi(t)\rangle = \mathrm{e}^{-iE_1 t} |\psi(0)\rangle$. On the other hand, the system is not in its ground state anymore after the pre-quench $\alpha_{\text{ini}} \to \alpha_{\text{int}}$. As a consequence, time evolution under $H(\alpha_{\text{int}})$, before the second quench $\alpha_{\text{int}} \to \alpha$ takes place, introduces a large set of different phases in the wavefunction, $|\psi(t)\rangle = \sum_n C_n \mathrm{e}^{-iE_n t} |\psi_n(\alpha_{\text{int}})\rangle$. These phases, that can be considered approximately random, are responsible for dephasing and thermalisation, and are also the origin of the erratic shape of the final energy distribution. As a consequence, we can consider that procedure (i) is somehow special, whereas procedure (ii) represents a more realistic situation in which many different time-dependent phases are present in the wavefunction.

### Dicke model

The Dicke model is used in the main text to show that two different trajectories, starting from the same initial states, can give rise to different statistics of work, if the initial states are not narrow enough in energy. So, the choice of the initial states is not so important as in the previous case. Hence, we have chosen a simple procedure, easy to implement. In all the cases, the initial state is a Fock state, $|\psi(0)\rangle = |m_j, n\rangle$, where $m_j = -j, \ldots, j$ is the projection of the total angular momentum $\vec{J}$ over the $z$ axis, and $n = 0, \ldots, n_{\text{max}}$ the number of photons. For any value of the coupling constant $\alpha$, the expected energy in such an initial state is

$$\frac{E(0)}{j} = \frac{1}{j} \langle\psi(0)| H_{\text{Dicke}} |\psi(0)\rangle = \omega_o \frac{m_j}{j} + \omega \frac{n}{j}. \quad (32)$$

This choice allows us to prepare initial states with energies $E_k/j = -1 + k/j$, with $k \in \mathbb{N} + \{0\}$. If $k < 2j$, we have $k+1$ different values of $m_j$ and $n$ for the same energy; if $k \geq 2j$, we have $2j+1$ different possibilities. Between all of them, we have always chosen the case for which the microcanonical averages gives the best description of the long-time averages of the four observables considered in the main text, $a^\dagger a$, $J_z$, $\left(a + a^\dagger\right)^2$, and $J_x^2$. It is worth noting that this procedure only allows to get initial states with energies larger than the critical of the ESQPT, $E/j = -1$. This fact does not constitute a problem, because we want to avoid the region with $E/j < -1$ because of its approximate integrability.

As it is shown in panel (b) Fig. 4 of the main text, the energy distribution resulting from this procedure is wide and erratic, similar to the coming from procedure (ii) in the LMG model. It is worth to comment that simple quenches give rise to similar energy distributions, contrary to what happens in the LMG model [22]. In this case, the main disadvantage of simple quenches is the integrable character of the Dicke model in the low-energy region, which can entail anomalous features in the energy distributions. So, we think that Fock initial states are better suited than simple quenches for the purpose of this work.

## THERMALISATION

In this section we discuss in detail the numerical calculations used in the main text to conclude that the initial states of both the LMG and Dicke models are properly thermalised.

### LMG model

#### *Calculations*

Equilibration and thermalisation are studied by means of long-time averages of representative observables. In all the cases discussed in the main text, we proceed in the following way:

*(i)* We let the system relax during a time $\tau = 10^8$ in the final Hamiltonian, $H(\alpha)$.

*(ii)* We compute all the observables at times $t_n = \tau + n\delta t$, with $\delta t = 10^3$, and $n = 0, 1, \ldots, 1000$.

*(iii)* We average over all these times, $\overline{\mathcal{O}} = \sum_{n=0}^{1000} \mathcal{O}(t_n)/N_t$, with $N_t = 1001$.

Results shown in panel (a) of Fig. 1 of the main text correspond to the observable $n_t/N$. In Fig. 8 we display the results for the four observables from which the finite-size scaling is obtained in the main text, $n_t/N$, and $Q \cdot Q/N^2$, $n_t^2/N^2$, and $n_t n_s/N^2$, evaluated at $t_n$, $\forall n$. In all the cases we see a good agreement between the analytical microcanonical average and the real time evolution, for initial states coming from both procedures. The quantitative analysis of this agreement shown in panel (b) of Fig. 1 in the main text is obtained from from time-averages described in point (iii) above, corroborating our conclusion.

#### *Eigenstate thermalisation hypothesis*

The ETH establishes that an isolated quantum system thermalises if the expected values of representative observables in the eigenstates of the Hamiltonian, $\langle E_n| \mathcal{O} |E_n\rangle$, are similar to the microcanonical average, $\text{Tr}\left[\rho(E, \alpha)\mathcal{O}\right]$,

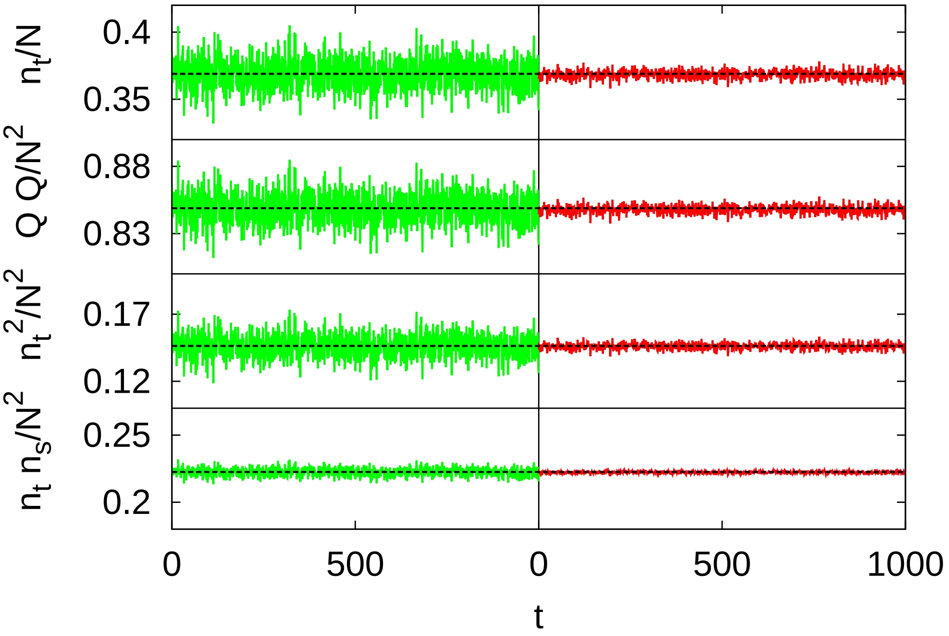


FIG. 8. Time-dependent expected values for $n_t/N$, $n_t^2/N^2$, $n_t n_s/N^2$ and $Q \cdot Q/N^2$ for the LMG model with $\alpha = 0.5$ and $E/N = -0.24$. Left column, states prepared following procedure (i) (see below and main text). Right column, states prepared following procedure (ii). Black dotted lines, analytical expected values, $\langle \mathcal{O}(E, \alpha) \rangle$. In all the cases, $N = 1, 6 \cdot 10^4$.

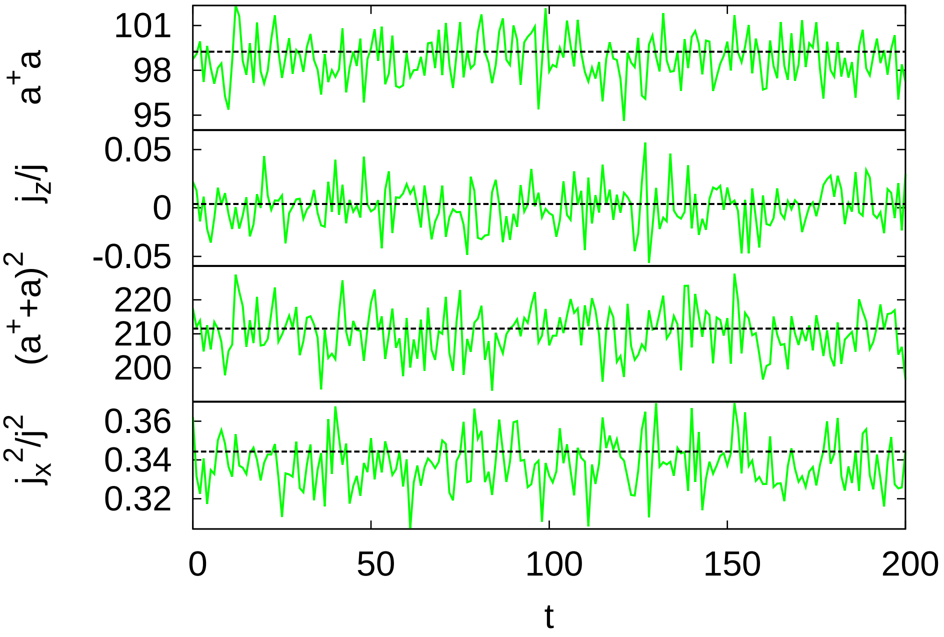


FIG. 9. Time-dependent expected values for $a^\dagger a$, $j_z/j$, $\left(a^\dagger + a\right)^2$ and $j_x^2/j^2$ for the Dicke model with $\alpha = 0.6$ and $E/j = 3.48$. Black dotted lines, microcanonical averages with a window of 51 energy levels. In all the cases, the number of atoms is $N = 50$, and the maximum number of photons is $n_{\max} = 700$.

within a small window $(E - \Delta E, E + \Delta E)$, where $E$ is the microcanonical energy. (A quantitative criterium, as a function of the energy width of the initial condition, is discussed in the main text). In Fig. 2 we plot the analytical results for the analytical microcanonical averages (solid line), together with the expected values in the corresponding

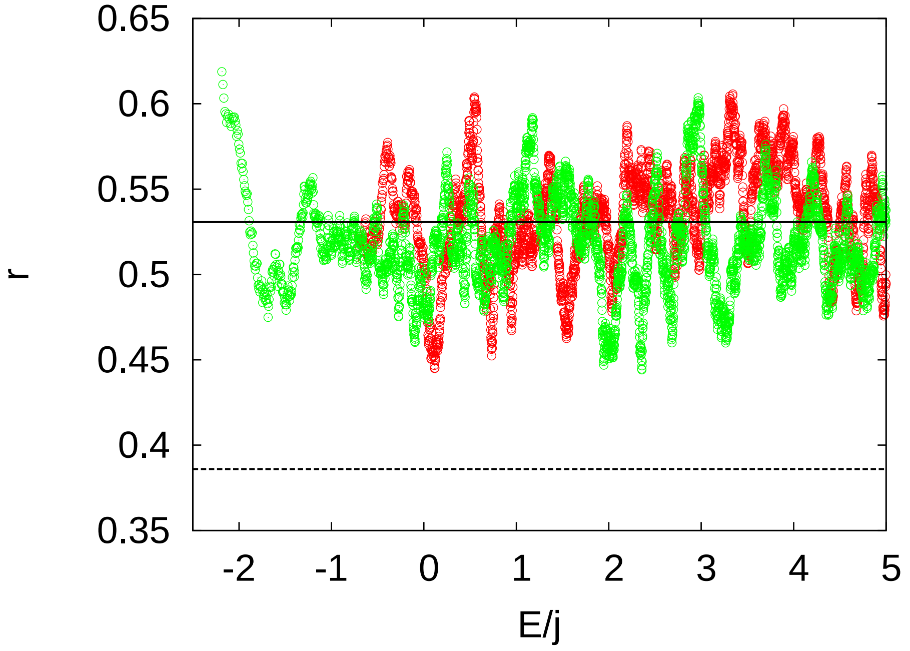


FIG. 10. Chaos parameter $r$, as a function of the energy for the Dicke model with $\alpha = 0.6$ (red symbols), and $\alpha = 1.2$ (green symbols). Solid black line, value of $r$ for a chaotic GOE-like spectrum. Dotted black line, value of $r$ for an integrable Poissonian spectrum. In all the cases, the number of atoms is $N = 50$, the maximum number of photons is $n_{\max} = 700$, and $\omega = \omega_o = 1$.

eigenstates, obtained with a system of size $N = 1,6 \cdot 10^4$, and $\alpha = 0.5$. We can see that the agreement between numerics and analytics is remarkable, even though the system has just one semiclassical degree of freedom and it is therefore integrable. All the calculated observables change smoothly with the energy, as required for the ETH to hold; only around the critical energy of the ESQPT, $E_c = 0$, do we see an abrupt behavior. Notwithstanding, it is worth to mention that the observables we have chosen are not artificially flat in energy —$n_t n_s / N^2$ and $Q \cdot Q/N^2$ decrease with energy for $E < 0$ with a remarkable slope. Therefore, the agreement between long-time averages coming from both procedures (i) and (ii), and the microcanonical averages is highly representative of thermalisation. Although not studied in this work, similar results are expected for other extensive observables not breaking the parity symmetry, like $n_t - n_s$ or $\left(s^\dagger t - t^\dagger s\right)^2$.

## Dicke model

### *Calculations*

The procedure is the same used with the LMG model. The only differences come from the relaxation time, in this case $\tau = 10^6$; the sampling time, $\delta t = 10^2$, and the number of sampled times, $N_t = 200$. This number is smaller than the one corresponding with the LMG model because calculations on the Dicke model require larger computational efforts.

Resuls for the observables studied in the main text are shown in Fig. 9, together with the quantum microcanonical average, done with 51 energy levels around the target energy. In all the calculations, $\omega = \omega_o = 1$, $\alpha = 0.6$, and $E/j = 3.48$ —the same values used in the main text. We see a very good agreement between the quantum microcanonical average and the real time evolution. It is worth noting that the size of the window used for the microcanonical average slightly affects the result. As we can see in Figs. 4 and 5, the expected values of the observables widely fluctuate around the quantum microcanonical average. As a consequence, the result of the average randomly depends on the window size, resulting in a slightly better or worse match between long-time and microcanonical averages. Notwidthstanding, this effect is small and expected to diminish as the number of atoms is increased. Unfortunately, it is not possible to perform a finite-size scaling analysis as it is done with the LMG model. Even though we have restricted ourselves to the possitive parity sector, the dimension of the Hilbert space in all the cases

discussed in the main text is around $d \sim 18000$. It is worth to comment that just storing the Hamiltonian matrix in double precision requires around 2.5 Gb of RAM memory. A system with $N = 100$ atoms in the same conditions would require around 40 Gb.

### *Eigenstate thermalisation hypothesis and chaos*

As the Dicke model has two degrees of freedom, a second constant of motion (besides the Hamiltonian itself) might exist, at least for certain values of the system parameters. For the classical version, such thing would entail that the trajectories would not explore the whole energy surface of the phase space, and hence the microcanonical average would not be correct. For the quantum version, a second constant of motion would imply the existence of a second quantum number to label the eigenstates. And this fact would entail that the expected values of physical observables would abruptly depend on the value of this second quantum number. This is observed in the low-energy region of the Dicke model with $\omega = \omega_o = 1$ and $\alpha = 1.2$. In Fig. 5 we can see a band structure below $E/j \sim -1$. As it is discussed in [17], each band correspond to a different value of a very approximate second integral of motion. Hence, thermalisation is not expected in this region. On the contrary, at energies larger than $E/j \sim -1$ for the case with $\alpha = 1.2$, and at all energies for the case with $\alpha = 0.6$, all the observables randomly fluctuate around the quantum microcanonical average. This is the reason why the region below $E/j \sim -1$ is avoided in the numerical experiments shown in the main text.

It is well known that there exists a link between quantum thermalisation and chaos —highly chaotic (ergodic) quantum systems are expected to fulfill all the requirements of the ETH. This is corroborated in Fig. 10. There, we display a signature of quantum chaos, based on spectral statistics —the average $\langle r \rangle$ of the quotient between two consequtive nearest-neighbour spacings, $s_n = E_n - E_{n-1}$, defined as [23]

$$r_n = \min\left(\frac{s_n}{s_{n-1}}, \frac{s_{n-1}}{s_n}\right). \tag{33}$$

The averages are calculated using 200 consecutive levels centered at the plotted energy. In the main text we give the average values around $E/j = -0.12$ for the case with $\alpha = 1.2$, and in the whole region $-0.4 \leq E/j \leq 4.2$, for the case with $\alpha = 0.6$. Here, we show how $\langle r \rangle$ depends on the energy, by averaging over 200 consequtive spacings around the target energy $E$. As references, we also display results for generic ergodic systems, $\langle r \rangle = 0.5307(1)$, and generic integrable systems, $\langle r \rangle = 2\ln 2 - 1 \sim 0.386$. We can see that both the cases with $\alpha = 0.6$ and $\alpha = 1.2$ are close to the result for generic ergodic systems. It is worth noting that $\langle r \rangle$ seems to be larger than the ergodic one for the almost-integrable region of the case with $\alpha = 1.2$, $E/j < -1$. This fact deserves further research, which is beyond the scope of this work.

## QUANTUM FLUCTUATION THEOREMS

### Two projective measurement scheme

Microcanonical QFT is tested in the main part of the manuscript following a two-projective measurement (TPM) scheme:

*(i)* The system is prepared in an initial state with particular values of the energy, $E$, and the system external parameter, $\alpha_i$, by means of any of the previously discussed procedures. As a consecuence, the real state of the sistem is pure, $|\psi(t)\rangle$.

*(ii)* A measurement of the energy is performed, obtaining $E_n(\alpha_i)$. As a consequence, the state of the system collapses onto the corresponding eigenstate of the Hamiltonian, $H(\alpha_i)$, $|\psi(t)\rangle \to |\psi_n(\alpha_i)\rangle$.

*(iii)* The non-equilibrium process, $\alpha_i \to \alpha_f$ is performed, starting from the previously collapsed state, $|\psi_n(\alpha_i)\rangle$.

*(iv)* A second measurement of the energy is performed, obtaining $E_m(\alpha_f)$.

*(v)* The work required to complete this process is calculated as $w = E_m(\alpha_f) - E_n(\alpha_i)$.

To complete the backward process, $\alpha_f \to \alpha_i$, we proceed following the same steps, (i)-(v), from an initial pure state, with energy $E+w$ and system parameter $\alpha_f$. Note that we require just one forward process, repeated over many different realizations; and a large number of different backward processes, each one starting from a different initial energy $E+w$, and each one repeated over many different realizations.

This TPM scheme can be simulated relying on one of the two following strategies:

*(a)* Randomly selecting the wavefunctions at which the state collapses, $|\psi_n(\alpha_i)\rangle$ and $|\psi_m(\alpha_f)\rangle$, according to the corresponding probability distributions. And repeating these numerical experiments many different times, in order to obtain significant statistics.

*(b)* Profiting from the knowledge of the transition probabilities, that can be calculated in advance, to avoid repeating the same numerical experiments over many different random realizations.

All the numerical results shown in the main text are obtained following the strategy (b). In other words, we have always followed this scheme:

*(i)* We calculate $N$ different forward processes, each one starting from a different eigenstate, $|\psi_n(\alpha_i)\rangle$.

*(ii)* For each one, we calculate the probability, $p_{mn}$, of each possible value of the work, $w_{mn} = E_m(\alpha_f) - E_n(\alpha_i)$, by $p_{mn} = |\langle\psi_m(\alpha_f)| U |\psi_n(\alpha_i)\rangle|^2$, where $U$ is the time-evolution operator. As it has been pointed above, if the procedure consists just in a single quench, as in all the numerical experiments done with the LMG model, this transition probability is $p_{mn} = |\langle\psi_n(\alpha_i)|\,\psi_m(\alpha_f)\rangle|^2$. Calculations for the Dicke model are a bit more complex, since the non-equilibrium protocol followed in all the numerical experiments consists in two quenches and an intermediate relaxing stage. In this case $U(t) = \exp[-iH(\alpha_f)\,t]\exp[-iH(\alpha_{\text{int}})\,\tau]$, where $\tau$ is the time the system spends in the intermediate stage, $H(\alpha_{\text{int}})$, and $t$ the time at which the second projective measurement takes place. Hence, writting the eigenstates of the initial Hamiltonian in an eigenbasis of the intermediate one, $|\psi_n(\alpha_i)\rangle = \sum_k V_k^n |\psi_k(\alpha_{\text{int}})\rangle$, and the eigenstates of the intermediate Hamiltonian in the eigenbasis of the final one, $|\psi_k(\alpha_{\text{int}})\rangle = \sum_j C_j^k |\psi_j(\alpha_f)\rangle$, we obtain $p_{mn} = \left|\sum_k V_k^n C_m^k \exp[-iE_k(\alpha_{\text{int}})\,\tau]\right|^2$, which logically depends on the eigenvalues of $H_{\text{int}}$ and on the amount of time the system spends on it, $\tau$. The matrices $w_{mn}$ and $p_{mn}$ contain the information required to describe the non-equilibrium process, $\alpha_i \to \alpha_f$, started from any initial state, and completed by means a TPM scheme.

*(iii)* The time-evolved state $|\psi(t)\rangle$ before the non-equilibrium process takes place is $|\psi(t)\rangle = \sum_c C_n \mathrm{e}^{-iE_n t} |\psi_n(\alpha_i)\rangle$. So, the probability of a work $w_{mn} = E_m(\alpha_f) - E_n(\alpha_i)$ is $|C_n|^2$ times the probability of the transition $|\psi_n(\alpha_i)\rangle \to |\psi_m(\alpha_f)\rangle$, $p_{mn}$. That is, $P(w_{mn}) = |C_n|^2 p_{mn}$. Hence, we obtain the distribution $P(w_{mn})$ directly from the matrix $p_{mn}$ coming from stage (ii) of this scheme, without performing a very large number of realizations. Furthermore, the computation of this matrix, the part of the scheme with the largest computational cost, is completed in advance, so the simulation of the same quench, $\alpha_i \to \alpha_f$, can be repeated starting from any initial state with a small computational cost. It is worth noting that calculation of the matrices $p_{mn}$ and $w_{mn}$ for each of the processes with the Dicke model requires full diagonalization of each Hamiltonian matrix. These calculations have been performed with the LAPACK library, and they required a few days of computation with an Intel Xeon 2.3 GHz.

### Numerical procedure

QFTs are derived from the assumption that the microscopic dynamics is reversible. This implies that the probability of investing a work $w_{mn} = E_m(\alpha_f) - E_n(\alpha_i)$ in the forward part of the protocol is exactly the same that the probability of retrieving the same amount of work in the backwards one, $P_f(E, w_{mn})/P_b(E + w_{mn}, -w_{mn}) = 1$. This implies that Eq. (1) of the main part of the manuscript,

$$\frac{P_f(E,\alpha_i,w)}{P_b(E+w,\alpha_f,-w)} = \frac{g(E+w,\alpha_f)}{g(E,\alpha_i)}, \tag{34}$$

is not a microscopic, but a macroscopic expression, coming from a statistical average over many different trajectories. If we assume that $E_m(\alpha_f) - E_n(\alpha_i) \neq E_p(\alpha_f) - E_q(\alpha_i)$, $\forall\, m, n \neq p, q$, each transition $|\psi_n(\alpha_i)\rangle \to |\psi_m(\alpha_f)\rangle$ requires a different value for the work, $w_{mn} \neq w_{pq}\ \forall\, m, n \neq p, q$. Hence, the best way to test the microcanonical quantum Crook's theorem is to proceed in the following way:

*(i)* We select a window $\Delta w$.

*(ii)* We consider that every transition $E_n(\alpha_i) \to E_m(\alpha_f)$ with $w - \Delta w/2 \leq w_{mn} \leq w + \Delta w/2$, gives rise to the same amount of *macroscopic* work, $w$. The size of this window, $\Delta w$, must be large enough to include a large set of different transitions, $E_n(\alpha_i) \to E_m(\alpha_f)$, and small enough to show no macroscopic differences within.

*(iii-A)* We build an histogram, $P(E, \alpha_i, w_j)$, with $N$ bins centered at $w_j$, $j = 1, \cdots, N$, and width $\Delta w$, accounting for all the transitions with work within $(w_j - \Delta w/2, w - j + \Delta w/2)$. In all the cases, the initial state has the same energy, $E$, and it is prepared by one of the previoulsy discussed procedures.

*(iii-B)* We proceed in a similar way for the backwards protocol. In this case, the histogram is obtained from $N$ different initial states with energies $E + w_j$, and each bin accounts for all the transitions involving a work $(-w_j - \Delta w/2, -w_j + \Delta w/2)$ and coming from the initial state with energy $E + w_j$. Again this state is prepared by one of the previously discussed procedures.

*(iv)* We test Eq. (1) of the main part of the manuscript by means of histograms of size $\Delta w$, and restricting ourselves to the values of $w$ for which the number of transitions $E_n(\alpha_i) \to E_m(\alpha_f)$ is large enough.

The results shown in Fig.2 of the main part of the manuscript, corresponding to the LMG model, are obtained with $\Delta w = 0.005$, and we restrict ourselves to the range $w \in [0.34, 0.46]$ to assure good statistics. Results in Fig. 3, corresponding to the Dicke model, are obtained with $\Delta w = 0.04$ and $w \in [-0.48, 4.32]$.

---

* armando.relano@fis.ucm.es


[1] M. Greiner, O. Mandel, T. W. Hänsch, and I. Bloch, Nature **419**, 51 (2002).
[2] C. Gross, T. Zibold, E. Nicklas, J. Esteve, and M. K. Oberthaler, Nature **464**, 1165 (2010); T. Zibold, E. Nicklas, C. Gross, and M. K. Oberthaler, Phys. Rev. Lett. **105**, 204101 (2010).
[3] M. Albiez, R. Gati, J. Fölling, S. Hunsmann, M. Cristiani, and M. K. Oberthaler, Phys. Rev. Lett. **95**, 010402 (2005).
[4] A. Trenkwalder, G. Spagnolli, G. Semeghini, S. Coop, M. Landini, P. Castiho, L. Pezzé, G. Modugno, M. Inguscio, A. Smerzi, and M. Fattori, Nat. Phys. **12**, 826 (2015).
[5] M. J. Martin, M. Bishof, M. D. Swallows, X. Zhang, C. Benko, J. von-Stecher, A. V. Gorshkov, A. M. Rey, and J. Ye, Science **341**, 632 (2013).
[6] C. S. Gerving, T. M. Hoang, M. Anquez, C. D. Hamley, and M. S. Chapman, Nat. Comm. **3**, 1169 (2012).
[7] S. Will, T. Best, U. Schneider, L. Hacermüller, D.-S. Lühmann, and I. Bloch, Nature **465**, 197 (2010).
[8] K. Baumann, C. Guerlin, F. Brennecke, and T. Esslinger, Nature **464**, 1301 (2010); K. Baumann, R. Mottl, F. Brennecke, and T. Esslinger, Phys. Rev. Lett. **107**, 140402 (2011).
[9] L. D'Alessio, Y. Kafri, A. Polkovnikov, and M. Rigol, Adv. Phys. **65**, 239 (2016).
[10] M. Srednicki, Phys. Rev. E **50**, 888 (1994).
[11] M. Perarnau-Llobet, E. Bäumer, K. V. Hovhannisyan, M. Huber, and A. Acin, Phys. Rev. Lett. **118**, 070601 (2017); M. Lostaglio, Phys. Rev. Lett. **120**, 040602 (2018).
[12] J. Vidal, J. M. Arias, J. Dukelsky, and J. E. García-Ramos, Phys. Rev. C **73**, 054305 (2006).
[13] A. Relaño, J. M. Arias, J. Dukelsky, J. E. García-Ramos, and P. Pérez-Fernández, Phys. Rev. A **78**, 060102(R) (2008).
[14] P. Pérez-Fernández, A. Relaño, J. M. Arias, J. Dukelsky, and J. E. García-Ramos, Phys. Rev. A **80**, 032111 (2009).
[15] R. Puebla and A. Relaño, Phys. Rev. E **92**, 012101 (2015).
[16] M. A. Bastarrachea-Magnani, S. Lerma-Hernández, and J. G. Hirsch, Phys. Rev. A **89**, 032101 (2016).
[17] A. Relaño, M. A. Bastarrachea-Magnani, and S. Lerma-Hernández, EPL **116**, 050005 (2016); M. A. Bastarrachea-Magnani, A. Relaño, S. Lerma-Hernández, B. López del Carpio, J. Chávez-Carlos, and J. Hirsch, J. Phys. A **50**, 144002 (2017).
[18] W. Buijsman, V. Gritsev, and R. Sprik, Phys. Rev. Lett. **118**, 080601 (2017).
[19] P. Stransky, M. Macek, and P. Cejnar, Ann. Phys. **345**, 73 (2014).
[20] T. Brandes, Phys. Rev. E **88**, 032133 (2013).
[21] M. A. Bastarrachea-Magnani, S. Lerma-Hernńdez, and J. G. Hirsch, J. Stat. Mech. (2016) 093105.
[22] C. M. Lóbez and A. Relaño, Phys. Rev. E **94**, 012140 (2016).
[23] Y. Y. Atas, E. Bogomolny, O. Giraud, and G. Roux, Phys. Rev. Lett. **110**, 084101 (2013).
